# Supplementary material for: TG-PSM: Tunable Greedy Packet Sequence Morphing Based on Trace Clustering
Source: arXiv:1904.05738 source file (2019-04-01)
Supplement: Supplementary file 1 [file Appendices.tex]

\documentclass[journal]{IEEEtran}

\usepackage{cite}
\usepackage{authblk}
\usepackage{xcolor}
\usepackage[draft]{todonotes}
\usepackage{nth}
\usepackage{amsmath}
\usepackage{booktabs}
\usepackage[ruled]{algorithm2e}
\usepackage{tabularx}
\usepackage{abstract}

\usepackage{fancyhdr}
\pagestyle{fancy}
\lhead{Appendix}

\hyphenation{op-tical net-works semi-conduc-tor}

\begin{document}

\begin{table*}[t]
\centering
\begin{tabular}{p{0.08\linewidth}p{0.08\linewidth}p{0.08\linewidth}p{0.08\linewidth}p{0.08\linewidth}p{0.08\linewidth}p{0.08\linewidth}p{0.08\linewidth}p{0.08\linewidth}p{0.08\linewidth}}
\hline
Scheme  & Dunn & CH & Silhouette & DB & Connectivity & APN & AD & ADM & FOM  \\
\hline
MBC8 &0.015 &590.60 &0.0866 &5.0296 &14905.6 &0.3511 &1310.9 &340.47 & 190.22\\
MBC9 &0.013 &667.17 &0.0461 &2.0431 &15536.7 &0.3191 &1263.4 &273.63 & 186.37\\
MBC10 &0.014 &693.73 &0.0382 &2.3909 &15650.4 &0.3892 &1240.4 &307.60 & 185.10\\
PAM8 &0.032 &2995.4 &0.1591 &1.7398 &5635.9 &0.3144 &935.31 &253.78 & 148.60\\
PAM9 &0.032 &2745.1 &0.1501 &1.7572 &6006.2 &0.2821 &909.32 &218.26 & 146.67\\
PAM10 &0.034 &2595.9 &0.1507 &1.6891 &6155.8 &0.3201 &899.86 &241.91 & 143.57\\
SOM8 &0.037 &3075.8 &0.1655 &1.0464 &5362.7 &0.2488 &914.23 &199.24 & 147.50\\
SOM9 &0.040 &2848.7 &0.1625 &0.8121 &5692.6 &0.2746 &904.06 &221.70 & 145.43\\
SOM10 &0.012 &2667.5 &0.1590 &1.0808 &6136.2 &0.2410 &879.49 &186.74 & 144.62\\
AGNES8 &0.0480 &2459.7 &0.1019 &2.1167 &5400.3 &0.5443 &1038.3 &439.59 & 155.76\\
AGNES9 &0.0480 &2274.9 &0.0981 &1.8142 &5728.5 &0.5616 &1024.2 &443.57 & 153.35\\
AGNES10 &0.0500 &2130.5 &0.1001 &1.8730 &5947.0 &0.5674 &1010.6 &441.70 & 151.69\\
DIANA8 &0.041 &2554.0 &0.1662 &1.7011 &4793.4 &0.1806 &951.31 &151.84 & 154.71\\
DIANA9 &0.042 &2263.9 &0.1637 &1.0694 &4826.6 &0.2047 &945.66 &158.32 & 152.40\\
DIANA10 &0.045 &2132.8 &0.1605 &0.9948 &5246.7 &0.2114 &931.54 &159.23 & 148.98\\
\hline 
\end{tabular} 
\newline
\caption{Comparison Between WF Defenses.OF refers to the features that defense tries to obfuscate.}
\label{CAM}
\end{table*}

%\section{Appendix II: Detailed Evaluation Results}
%Detailed Evaluation Results are shown in Tables VI to XIV.

\begin{table*}[t]
\centering
\begin{tabular}{p{0.15\linewidth}p{0.35\linewidth}p{0.15\linewidth}p{0.15\linewidth}}
\hline
Countermeasure & Parameter & overhead & Classifier Accuracy \\
\hline
Traffic Morphing & SimThresh = 0.7 & 62.6 & $55.46\pm2.2$ \\
BuFLO & $\tau=0, \rho=40, d=1000$ & $100$ & $40.6\pm3.1$ \\
BuFLO & $\tau=0, \rho=20, d=1500$ & $151$ & $31.2\pm2.8$ \\
BuFLO & $\tau=10000, \rho=40, d=1000$ & $131.7$ & $28.1\pm1.4$ \\
BuFLO & $\tau=10000, \rho=20, d=1000$ & $277$ & $10.9\pm0.8$\\
TAMARAW & $L_1$ & $79.2$ & $26.7\pm2.2$ \\
TAMARAW & $L_2$ & $225.6$ & $9.7\pm1.5$ \\
TGPSM & $D=1$ & $86.5$ & $23.43\pm1.2$ \\
TGPSM & $D=3$ & $125$ & $21.26\pm0.8$ \\
TGPSM & $D=5$ & $135.6$ & $18.6\pm1.4$ \\
TGPSM & $D=7$ & $144$ & $17.1\pm0.9$ \\
TGPSM & $D=9$ & $158$ & $13.2\pm1.1$ \\
\hline
\end{tabular} 
\newline
\caption{Overhead and accuracy results for different countermeasures against LL classifier at k=32 on Herrmann dataset}
\label{LLK32Results}
\end{table*}

\begin{table*}[t]
\centering
\begin{tabular}{p{0.15\linewidth}p{0.35\linewidth}p{0.15\linewidth}p{0.15\linewidth}}
\hline
Countermeasure & Parameter & overhead & Classifier Accuracy \\
\hline
Traffic Morphing & SimThresh = 0.7 & 56.7 & $17.7$ \\
BuFLO & $\tau=0, \rho=40, d=1000$ & $103$ & $6.5\pm2.4$ \\
BuFLO & $\tau=0, \rho=20, d=1500$ & $149$ & $6.3\pm1.2$ \\
BuFLO & $\tau=10000, \rho=40, d=1000$ & $131.2$ & $3.4\pm4.3$ \\
BuFLO & $\tau=10000, \rho=20, d=1000$ & $269$ & $2.4\pm0.5$\\
TAMARAW & $L_1$ & $79.2$ & $2.8\pm2.5$ \\
TAMARAW & $L_2$ & $225.6$ & $1\pm0.8$ \\
TGPSM & $D=1$ & $88.3$ & $8.0\pm1.1$ \\
TGPSM & $D=3$ & $119.4$ & $6.2\pm0.7$ \\
TGPSM & $D=5$ & $129.6$ & $3.2\pm1.2$ \\
TGPSM & $D=7$ & $137.7$ & $1\pm0.8$ \\
TGPSM & $D=9$ & $149.2$ & $1\pm0.8$ \\
\end{tabular} 
\newline
\caption{Overhead and accuracy results for different countermeasures against HA classifier at k=32 on Herrmann dataset}
\label{HAK32Results}
\end{table*}

\begin{table*}[t]
\centering
\begin{tabular}{p{0.15\linewidth}p{0.35\linewidth}p{0.15\linewidth}p{0.15\linewidth}}
\hline
Countermeasure & Parameter & overhead & Classifier Accuracy \\
\hline
Traffic Morphing & SimThresh = 0.7 & 56 & $92.3\pm0.8$ \\
BuFLO & $\tau=0, \rho=40, d=1000$ & $96$ & $63.8\pm1.5$ \\
BuFLO & $\tau=0, \rho=20, d=1500$ & $137$ & $59.4\pm0.8$ \\
BuFLO & $\tau=10000, \rho=40, d=1000$ & $132$ & $48.9\pm1.8$ \\
BuFLO & $\tau=10000, \rho=20, d=1000$ & $287.1$ & $35.7\pm0.6$ \\
TAMARAW & $L_1$ & $84.6$ & $39.2\pm1.2$ \\
TAMARAW & $L_2$ & $256$ & $24.8\pm2.2$ \\
TGPSM & $D=1$ & $87$ & $47.1\pm0.7$ \\
TGPSM & $D=3$ & $124.3$ & $43.6\pm2.2$ \\
TGPSM & $D=5$ & $135.7$ & $31.5\pm3.1$ \\
TGPSM & $D=7$ & $142.1$ & $25.4\pm2.4$ \\
TGPSM & $D=9$ & $161.3$ & $19.2\pm1.3$ \\
\hline
\end{tabular} 
\newline
\caption{Overhead and accuracy results for different countermeasures against PA classifier at k=32 on Herrmann dataset}
\label{PAK32Results}
\end{table*}

\end{document}
